# Supplementary material for: Measurement of the helicity-dependent response in quasi-elastic proton knockout from $^{40}{\rm Ca}$
Source: arXiv:2504.09972 source file (2025-04-14)
Supplement: Supplementary file 1 [file 5th_Calcium_SupplementaryMaterial-arxiv.pdf]

# Measurement of the helicity-dependent response in quasi-elastic proton knockout from $^{40}$Ca

## Supplementary material

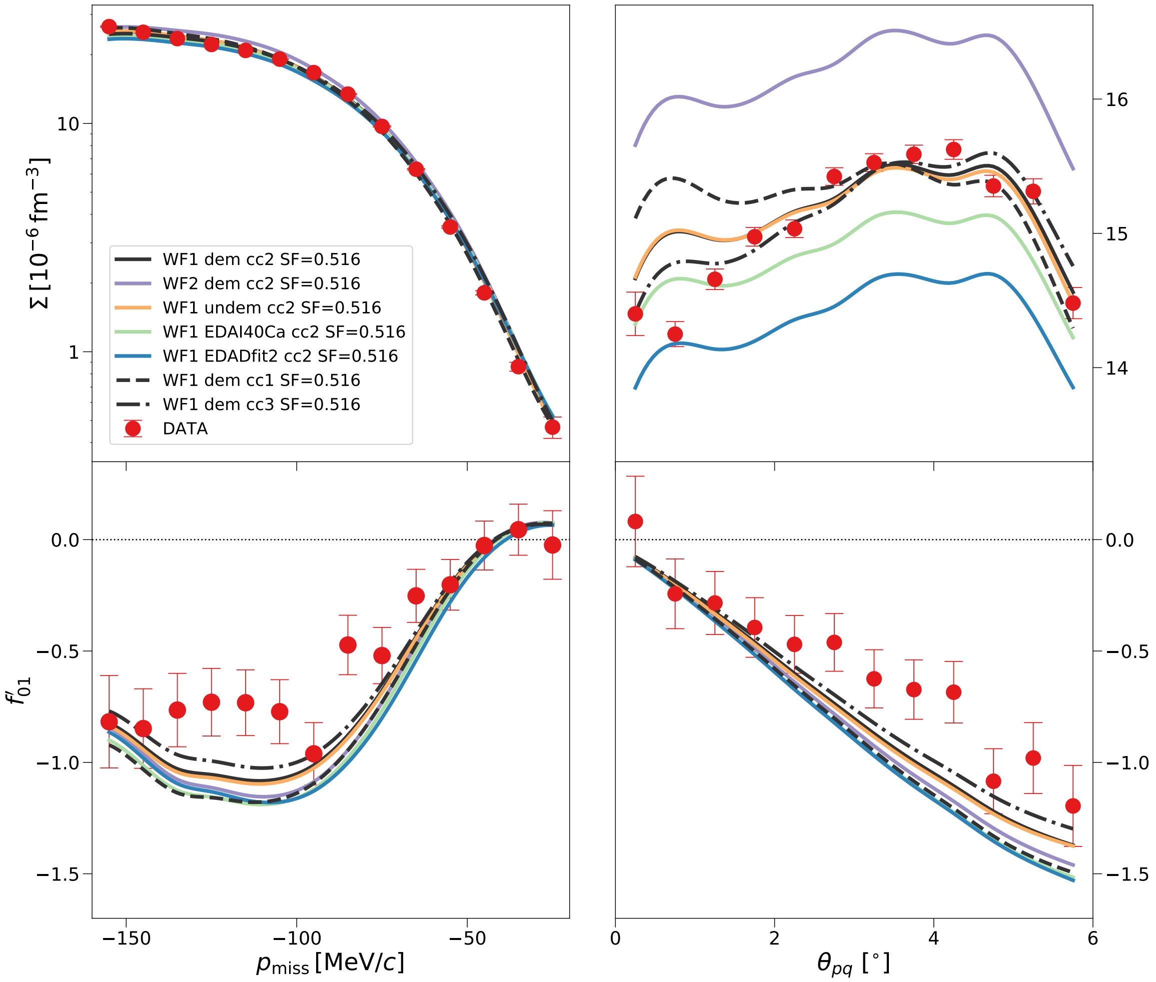


Figure S1: Shown are data and RDWIA calculations [1] for the unpolarized cross section (*top*) and the fifth structure function (*bottom*) as a function of the missing momentum (*left*) and the polar angle between the outgoing proton and the momentum transfer (*right*). All calculations are shown with the same spectroscopic factor (SF) which was obtained by comparing missing momentum distribution of data and the RDWIA calculation (WF1 dem cc2) that uses the democratic optical potential [2], the bound-state wave function from Ref. [3], the *cc2* prescription for the nuclear current from Ref. [4], and the free-proton electromagnetic form factors from Ref. [5]. We used i) three alternative parameterizations of the relativistic optical potential; undemocratic fit [2], Energy-Dependent A-Independent (EDAI) fit to $^{40}$Ca data and Energy-Dependent A-Dependent (EDAD) fit [6], ii) another bound-state wavefunction [7], and iii) different off-shell nuclear current prescriptions (*cc1*, *cc3*) [4]. For $f'_{01}$ the variation of these calculations is shown by a gray band in bottom panels in Figs. 4 and 5 of the main article.

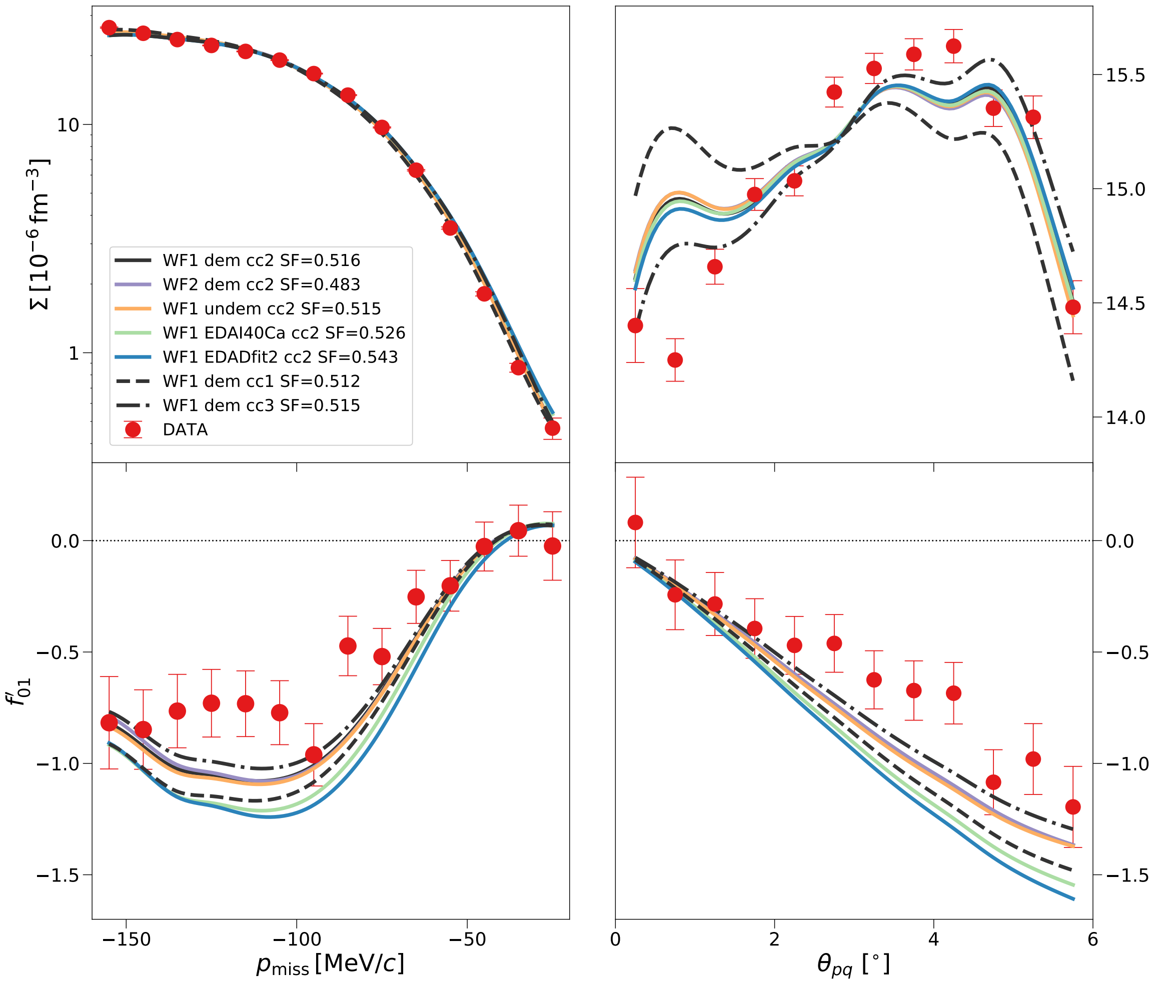


Figure S2: Same as Fig. S1 but with each calculation independently fitted to missing momentum distribution of unpolarized cross section, resulting in slight variations in spectroscopic factors (SF).

## References


[1] A. Meucci, C. Giusti, F. D. Pacati, Relativistic corrections in $(e, e'p)$ knockout reactions, Phys. Rev. C 64 (2001) 014604. arXiv:nucl-th/0101034, doi:10.1103/PhysRevC.64.014604.

[2] E. D. Cooper, S. Hama, B. C. Clark, Global dirac optical potential from helium to lead, Phys. Rev. C 80 (2009) 034605. doi:10.1103/PhysRevC.80.034605.

[3] M. Sharma, M. Nagarajan, P. Ring, Rho meson coupling in the relativistic mean field theory and description of exotic nuclei, Phys. Lett. B 312 (4) (1993) 377 – 381. doi:https://doi.org/10.1016/0370-2693(93)90970-S.

[4] T. De Forest, Off-shell electron-nucleon cross sections: The impulse approximation, Nucl. Phys. A 392 (2) (1983) 232 – 248. doi:https://doi.org/10.1016/0375-9474(83)90124-0.

[5] J. C. Bernauer, M. O. Distler, J. Friedrich, T. Walcher, P. Achenbach, C. Ayerbe-Gayoso, et al., Electric and magnetic form factors of the proton, Phys. Rev. C 90 (1) (2014) 015206. doi:10.1103/PhysRevC.90.015206.

[6] E. D. Cooper, S. Hama, B. C. Clark, R. L. Mercer, Global Dirac phenomenology for proton nucleus elastic scattering, Phys. Rev. C 47 (1993) 297–311. doi:10.1103/PhysRevC.47.297.

[7] G. A. Lalazissis, J. Konig, P. Ring, A New parametrization for the Lagrangian density of relativistic mean field theory, Phys. Rev. C 55 (1997) 540–543. arXiv:nucl-th/9607039, doi:10.1103/PhysRevC.55.540.
